# Supplementary material for: Learning dynamics on the picosecond timescale in a superconducting synapse structure
Source: arXiv:2504.02754 source file (2025-04-03)
Supplement: Supplementary file 1 [file Supplemental_Material.pdf]

# Supplemental Material

**Learning dynamics on the picosecond timescale in a superconducting synapse structure**

K. Segall, L. Nichols, W. Friend and S.B. Kaplan

Contents | Page

1. Construction of voltage 3-D color plots. . . . . . . 2
2. Equivalence of $V_{top}$, $V_{bot}$, and $V_{neuron}$ . . . . . . . 3
3. Circuit details and experimental parameters . . . . . . 4

## 1. Construction of 3-D color plots

This section discusses the construction of 3-D color plots for experimental data, used in the manuscript for Figs. 2a, 3, and 6a. In all of these plots there are two applied currents, plotted on the x- and y-axes, and one measured voltage, plotted on the z-axis using a color scale. In the example below, we describe the formation of Fig. 2a, where the two currents are the neuron input current and the neuron bias current and the voltage is the top JTL voltage. The other two figures are similar: Fig. 3 switches the SQUID voltage for the top JTL voltage, while Fig. 6a switches the top JTL current for the neuron bias current. In Fig. 2a and Fig. 6a the voltage is displayed as a spiking frequency via the Josephson relationship.

The basic scheme is to use an AC sawtooth current for the neuron input and a DC current for the neuron bias. The sawtooth current is produced by a function generator at around 100 Hz and is coupled into our balanced bias circuit through a transformer to help separate grounds. The value of this AC current is measured by an instrumentation amplifier across a sense resistor in series with the neuron. Meanwhile the DC current for the neuron bias is produced by a programmable DC voltage across a large series resistor. Fig. S1a shows the electrical diagram, and Fig. S1b shows the measured input current versus time.

The voltage is measured simultaneously with the current application. The left side of Fig. S2 shows the top JTL voltage versus input current for two different values of the neuron bias current. These plots are averaged over 500 periods and then assembled as “slices” in the color plot, shown on the right side of Fig. S2. The z-axis for the plot below is in microvolts; it can be converted to a spiking frequency via the Josephson relation if desired. (Note: This plot shows a larger range of input current than Fig. 2a; since it was periodic we chose to show a smaller range in more detail in the manuscript.)

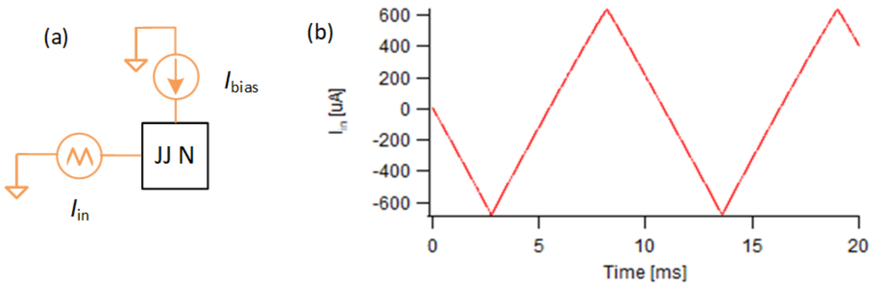


*Fig. S1: Current biasing for color plots. (a) Circuit diagram, showing that the input current $I_{in}$ is an AC wave in a sawtooth shape while the bias current $I_{bias}$ is a DC current. (b) Input current versus time, showing the sawtooth wave at 100 Hz.*

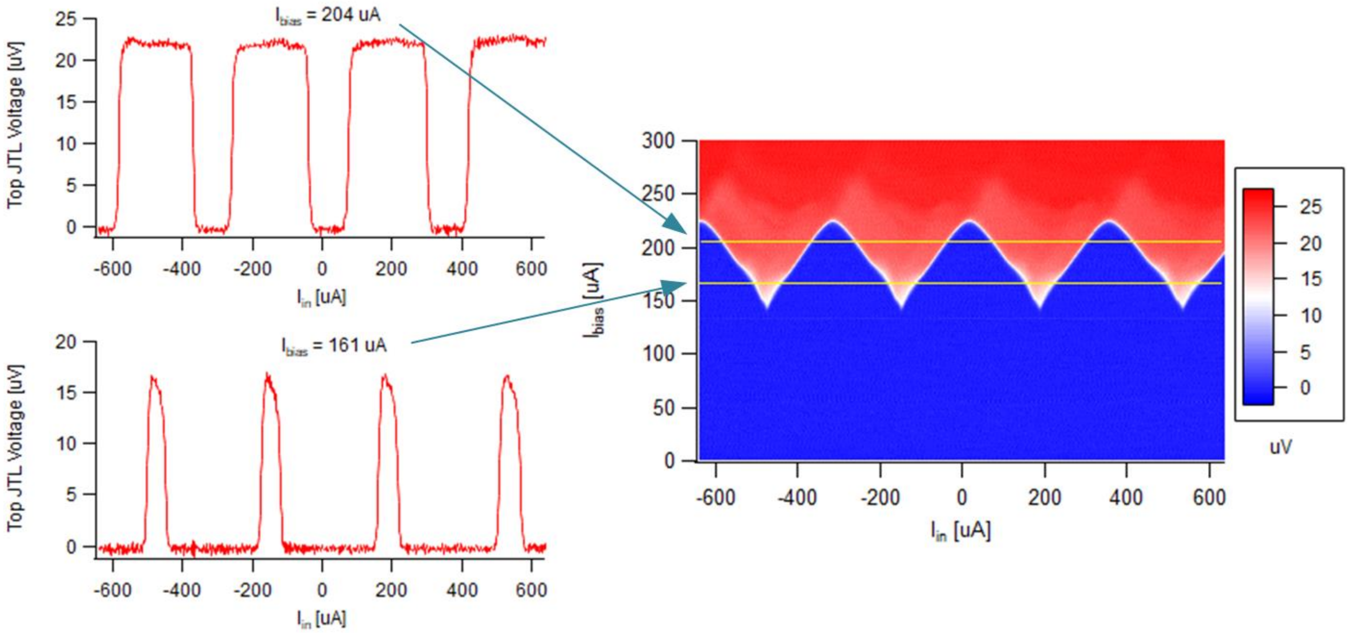


*Fig. S2: Formation of the color plot from slices of constant $I_{bias}$. Left: Two slices of top JTL voltage at $I_{bias}$ = 161 $\mu$A and 204 $\mu$A. Right: Color plot of $V_{top}$, with the two yellow lines showing the location of the two slices.*

## 2. Equivalence of $V_{\text{top}}$, $V_{\text{bot}}$, and $V_{\text{neuron}}$

This section shows data to support the claim that under the conditions of properly biased JTLs, the voltage across the top JTL ($V_{\text{top}}$), the bottom JTL ($V_{\text{bot}}$), and the neuron ($V_{\text{neuron}}$) are the same for all values of neuron bias and neuron input. The voltages are converted to pulsing frequencies via the Josephson relationship. Fig. S3 shows the color plots of the pulsing frequency of the neuron and the bottom JTL. These plots are indistinguishable by eye from Fig. 2a in the manuscript.

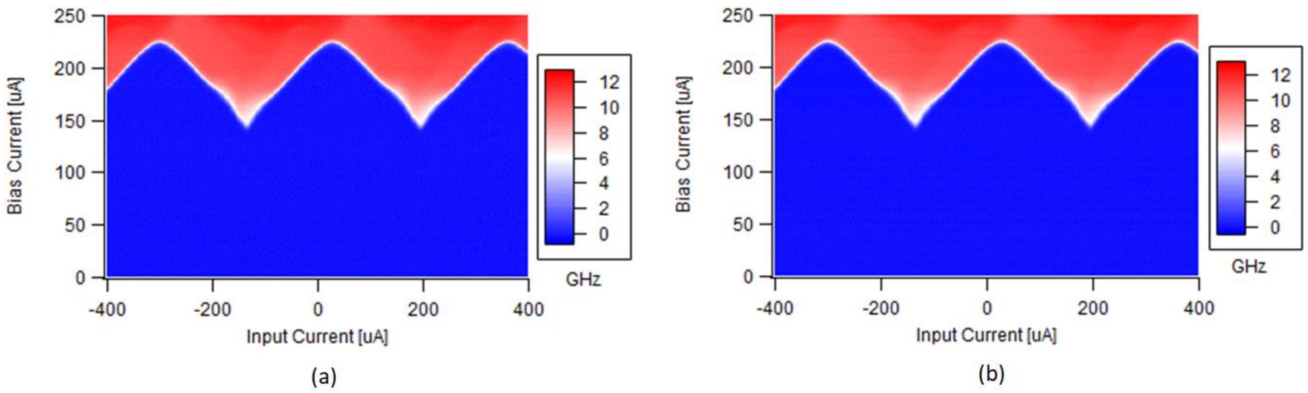


*Fig. S3: Color plots of the spiking frequency of (a) the bottom JTL (b) the neuron. These plots are indistinguishable from Fig. 2a in the manuscript.*

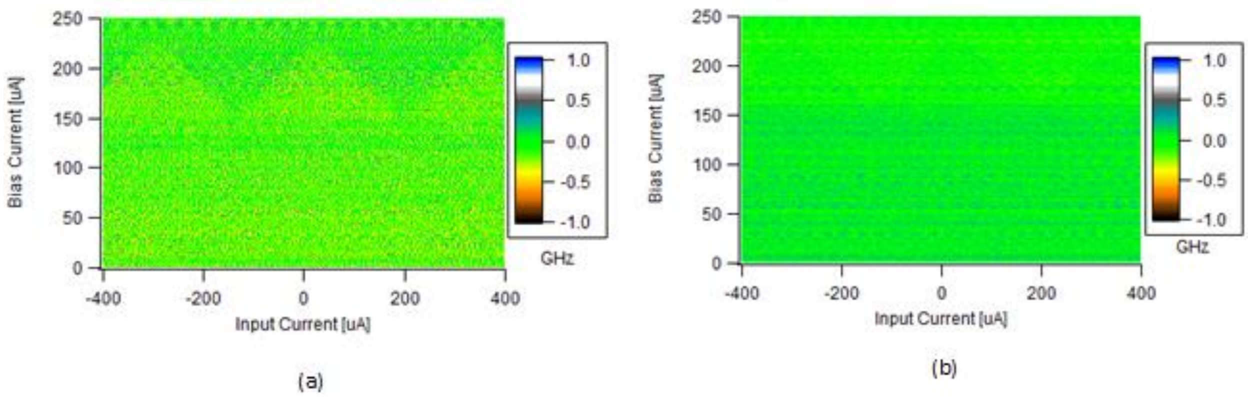


*Fig S4: Color plot of the difference in spiking frequency of (a) the bottom JTL and the top JTL, and (b) the neuron and the top JTL. The plots are essentially zero for all points, to within 0.2 GHz.*

In Fig. S4 we show a color plot of the difference in spiking frequency between the bottom JTL and the top JTL (left), and the neuron and the top JTL (right). The plots are almost entirely green, showing that the difference is essentially zero in both cases, to within a standard deviation of about 0.2 GHz. The full statistical comparison for all 250,000 points in all of the 3-D plots is given in Table 1.

| | Average [GHz] | Standard Deviation [GHz] |
|---|---|---|
| Bottom JTL minus Top JTL | -0.12 | 0.19 |
| Neuron minus Top JTL | 0.01 | 0.16 |
| Neuron minus Bottom JTL | 0.13 | 0.09 |

*Table 1: Statistical comparison of the spiking frequency of the bottom JTL, top JTL and neuron*

### 3. Circuit details and experimental parameters

In this section we give two tables of information for the circuit parameters and the experimental values of the currents used in the figures. Table 2 gives the critical currents, shunt resistors and inductances for the various parts of the circuit while Table 3 gives the applied currents for the figures in the paper.

| | **# of Junctions** | **Critical currents** | **Shunt resistors** | **Inductances** |
|---|---|---|---|---|
| JJ neuron | 2 | 109 μA | 1.3 Ω | 12.5 pH |
| Top JTL | 21 | 75 μA | 3.9 Ω | 18.5 pH |
| Bottom JTL | 7 | 68 - 109 μA | 2.2-3.9 Ω | 7.2-12.8 pH |
| Learning gate | 2 | 83 μA, 109 μA | 1.8 Ω, 2.4 Ω | 8 pH, 12 pH |
| Memory loop | 1 | 109 μA | 1.8 Ω | 19.3 nH |
| SQUID | 2 | 110 μA | 1.3 Ω | 7.7 pH |

*Table 2: Critical currents, inductances and shunt resistances for the different parts of the circuit*

| | **Fig. 2a, Fig. 3, Fig. S1-S4** | **Fig. 6a, Fig. 8** |
|---|---|---|
| $I_{in}$ | -600 to 600 μA | -200 to 200 μA |
| $I_{bias}$ | 0 to 250 μA | 190 μA |
| $I_{top}$ | 616 μA | 500-640 μA |
| $I_{bot}$ | 318.5 μA | 322 μA |
| $I_{mem}$ | 129 μA | 119 μA |
| $I_{LG}$ | 132 μA | 118 μA |
| $I_{SQ}$ | 285 μA | 279 μA |

*Table 3: Bias currents for the figures in the manuscript*
